# Supplementary material for: Distinguishing Artificial and Essential Symmetry Breaking in a Single Determinant: Approach and Application to the C$_{60}$, C$_{36}$, and C$_{20}$ Fullerenes
Source: arXiv:1812.05266 source file (2018-12-13)
Supplement: Supplementary file 1 [file jp5b10266_si_001.pdf]

# What are the Ground State Structures of $C_{20}$ and $C_{24}$? An Explicitly Correlated *Ab initio* Approach

Debashree Manna and Jan M.L. Martin*
*Department of Organic Chemistry, Weizmann Institute of Science, 76100 Reḥovot, Israel. Email: gershom@weizmann.ac.il*

## Supporting Information

**Table S1** Relative energies (kcal/mol) calculated using various *ab initio* methods for different $C_{20}$ and $C_{24}$ isomers using the cc-pVDZ basis set

| Structure/VDZ | HF | MP2 | MP2-HF | MP3 | MP2.5[a] | CCSD | CCSD(T) | MP2.5-MP2 | CCSD-HF | just (T) | CCSD(T)-MP2.5 | HLC[b] |
|---|---|---|---|---|---|---|---|---|---|---|---|---|
| $C_{20}$ Bowl $C_{5v}$ | 0.00 | 0.00 | 0.00 | 0.00 | 0.00 | 0.00 | 0.00 | 0.00 | 0.00 | 0.00 | 0.00 | 0.00 |
| $C_{20}$ Cage $C_{2h}$ | 53.53 | -18.88 | -72.41 | 29.01 | 5.07 | 21.94 | 7.05 | 23.94 | -31.59 | -14.89 | 1.98 | 25.92 |
| $C_{20}$ Cage $C_i$ | 53.92 | -19.73 | -73.66 | 28.34 | 4.31 | 21.44 | 6.58 | 24.04 | -32.48 | -14.86 | 2.28 | 26.31 |
| $C_{20}$ Cage $D_{2h}$ | 53.54 | -18.89 | -72.43 | 29.00 | 5.05 | 21.93 | 7.03 | 23.95 | -31.61 | -14.90 | 1.97 | 25.92 |
| $C_{20}$ Cage $D_{3h}$ | 53.91 | -19.72 | -73.63 | 28.30 | 4.29 | 21.43 | 6.58 | 24.01 | -32.49 | -14.85 | 2.29 | 26.30 |
| $C_{20}$ Ring $C_{10h}$ | -8.57 | 56.55 | 65.12 | 45.15 | 50.85 | 45.36 | 54.26 | -5.70 | 53.93 | 8.91 | 3.41 | -2.28 |
| $C_{24}$ Cage $O_h$ | 47.01 | 33.05 | -13.95 | 24.01 | 28.53 | 30.34 | 27.57 | -4.52 | -16.66 | -2.77 | -0.96 | -5.48 |
| $C_{24}$ Cage $D_{3d}$ | 21.93 | -11.95 | -33.88 | -8.09 | -10.02 | -5.55 | -11.53 | 1.93 | -27.48 | -5.97 | -1.50 | 0.43 |
| $C_{24}$ Corona $D_{6h}$ | 0.00 | 0.00 | 0.00 | 0.00 | 0.00 | 0.00 | 0.00 | 0.00 | 0.00 | 0.00 | 0.00 | 0.00 |
| $C_{24}$ Ring $C_{12h}$ | 20.22 | 90.70 | 70.48 | 82.95 | 86.82 | 81.25 | 91.76 | -3.88 | 61.03 | 10.50 | 4.93 | 1.06 |

[a] MP2.5= (MP2+MP3)/2
[b]HLC=CCSD(T)-MP2)

**Table S2** Relative energies (kcal/mol) calculated using various *ab initio* methods for different $C_{20}$ and $C_{24}$ isomers using the cc-pV5Z basis set

| Structure/V5Z | HF | MP2 | MP2-HF |
|---|---|---|---|
| $C_{20}$ Bowl $C_{5v}$ | 0.00 | 0.00 | 0.00 |
| $C_{20}$ Cage $C_{2h}$ | ---[a] | ---[a] | ---[a] |
| $C_{20}$ Cage $C_i$ | ---[a] | ---[a] | ---[a] |
| $C_{20}$ Cage $D_{2h}$ | 66.16 | -16.99 | -83.15 |
| $C_{20}$ Cage $D_{3h}$ | ---[a] | ---[a] | ---[a] |
| $C_{20}$ Ring $C_{10h}$ | -20.05 | 49.96 | 70.01 |
| $C_{24}$ Cage $O_h$ | ---[a] | ---[a] | ---[a] |
| $C_{24}$ Cage $D_{3d}$ | 39.05 | -4.21 | -43.27 |
| $C_{24}$ Corona $D_{6h}$ | 0.00 | 0.00 | 0.00 |
| $C_{24}$ Ring $C_{12h}$ | 8.98 | 86.00 | 77.02 |

[a]Values are not reported due to a convergence problem.

**Table S3** MP2-pwCVQZ calculated core-valence contribution (kcal/mol)

| Structure | Relative Energy Valence | Relative Energy All electron | core-valence contribution |
|---|---|---|---|
| $C_{20}$ Bowl $C_{5v}$ | 0.00 | 0.00 | 0.00 |
| $C_{20}$ Cage $C_{2h}$ | ---[a] | ---[a] | ---[a] |
| $C_{20}$ Cage $C_i$ | ---[a] | ---[a] | ---[a] |
| $C_{20}$ Cage $D_{2h}$ | -14.75 | -13.82 | 0.94 |
| $C_{20}$ Cage $D_{3h}$ | -15.61 | -14.69 | 0.92 |
| $C_{20}$ Ring $C_{10h}$ | 48.99 | 47.91 | -1.08 |
| $C_{24}$ Cage $O_h$ | ---[a] | ---[a] | ---[a] |
| $C_{24}$ Cage $D_{3d}$ | -1.98 | -0.85 | 1.12 |
| $C_{24}$ Corona $D_{6h}$ | 0.00 | 0.00 | 0.00 |
| $C_{24}$ Ring $C_{12h}$ | ---[a] | ---[a] | ---[a] |

[a]Values are not reported due to a convergence problem.

**Table S4** DFT Relative energies (kcal/mol) for various $C_{22}$ isomers using the def2-TZVPP basis set

| Structure | PBE0/def2-TZVPP | DSD-PBEP86-D3BJ-TZVPP |
|---|---|---|
| $C_{22}$ Cage $C_2$ | 0.00 | 0.00 |
| $C_{22}$ Cage $C_1$ | 5.84 | 7.52 |
| $C_{22}$ Cage $C_s$ | 10.60 | 11.09 |
| $C_{22}$ Cage $C_2'$ | 15.54 | 17.33 |
| $C_{22}$ Bowl $C_{2v}$ | 36.62 | 37.49 |
| $C_{22}$ Ring $C_{11h}$ | 14.64 | 22.98 |

Table S5 Relative Gibbs free energies ($E_T$) (kcal/mol) with MP2-F12/VTZ-F12+HLC/VTZ at very high temperature range (500-3000K) for various $C_{20}$ and $C_{24}$ isomers

| Structure | $E_{298}$ | $E_{500}$ | $E_{1000}$ | $E_{1500}$ | $E_{2000}$ | $E_{2500}$ | $E_{3000}$ |
|---|---|---|---|---|---|---|---|
| $C_{20}$ Bowl $C_{5v}$ | 0.00 | 0.00 | 0.00 | 0.00 | 0.00 | 0.00 | 0.00 |
| $C_{20}$ Cage $C_{2h}$ | ---[a] | ---[a] | ---[a] | ---[a] | ---[a] | ---[a] | ---[a] |
| $C_{20}$ Cage $C_i$ | ---[a] | ---[a] | ---[a] | ---[a] | ---[a] | ---[a] | ---[a] |
| $C_{20}$ Cage $D_{2h}$ | 13.47 | 16.19 | 24.17 | 32.26 | 40.30 | 48.31 | 56.30 |
| $C_{20}$ Cage $D_{3d}$ | 12.13 | 14.28 | 20.82 | 27.47 | 34.07 | 40.63 | 47.18 |
| $C_{20}$ Ring $C_{10h}$ | 33.75 | 26.64 | 6.91 | -13.19 | -33.28 | -53.33 | -73.37 |
| $C_{24}$ Cage $O_h$ | 41.03 | 47.10 | 63.68 | 80.42 | 97.12 | 113.77 | 130.41 |
| $C_{24}$ Cage $D_{3d}$ | 4.76 | 10.64 | 26.97 | 43.54 | 60.07 | 76.58 | 93.06 |
| $C_{24}$ Corona $D_{6h}$ | 0.00 | 0.00 | 0.00 | 0.00 | 0.00 | 0.00 | 0.00 |
| $C_{24}$ Ring $C_{12h}$ | 71.18 | 63.62 | 42.62 | 21.23 | -0.14 | -21.48 | -42.80 |

[a]Values are not reported due to a convergence problem.

**Table S6** Smallest Eigenvalues for the different $C_{20}$ and $C_{24}$ isomers using the cc-pVDZ-F12 and cc-pVTZ-F12 basis set

| Structure | cc-pVDZ-F12 | cc-pVTZ-F12 |
|---|---|---|
| $C_{20}$ Bowl $C_{5v}$ | 0.191E-07 | 0.811E-08 |
| $C_{20}$ Cage $C_{2h}$ | 0.451E-06 | 0.219E-06 |
| $C_{20}$ Cage $C_i$ | 0.465E-06 | 0.224E-06 |
| $C_{20}$ Cage $D_{2h}$ | 0.452E-06 | 0.219E-06 |
| $C_{20}$ Cage $D_{3d}$ | 0.465E-06 | 0.224E-06 |
| $C_{20}$ Ring $C_{10h}$ | 0.196E-09 | 0.961E-10 |
| $C_{24}$ Cage $O_h$ | 0.635E-08 | 0.256E-08 |
| $C_{24}$ Cage $D_{3d}$ | 0.746E-07 | 0.349E-07 |
| $C_{24}$ Corona $D_{6h}$ | 0.545E-09 | 0.171E-09 |
| $C_{24}$ Ring $C_{12h}$ | 0.530E-10 | 0.181E-10 |

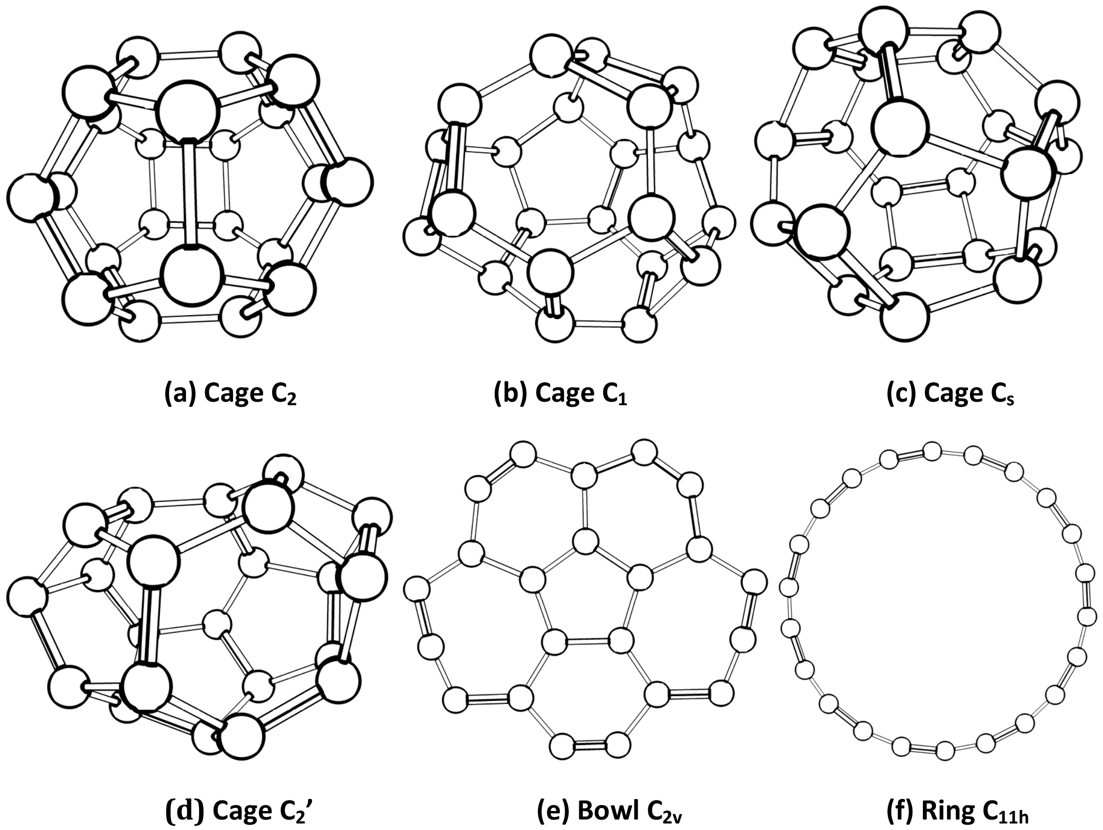


**Figure S1** Structures of the six $C_{22}$ isomers.

**Cartesian coordinates:**

$C_{20}$ Bowl $C_{5v}$

| | | | |
|---|---|---|---|
| C | 0.000000 | 1.208204 | 0.462774 |
| C | -1.149070 | 0.373356 | 0.462774 |
| C | 1.149070 | 0.373356 | 0.462774 |
| C | -0.710164 | -0.977457 | 0.462774 |
| C | 0.710164 | -0.977457 | 0.462774 |
| C | 0.000000 | 2.555215 | 0.012600 |
| C | -2.430154 | 0.789605 | 0.012600 |
| C | 2.430154 | 0.789605 | 0.012600 |
| C | -1.501918 | -2.067212 | 0.012600 |
| C | 1.501918 | -2.067212 | 0.012600 |
| C | 1.343182 | 2.901210 | -0.237687 |
| C | -3.174281 | -0.380919 | -0.237687 |
| C | 2.344148 | 2.173965 | -0.237687 |
| C | -2.791945 | -1.557625 | -0.237687 |
| C | 3.174281 | -0.380919 | -0.237687 |
| C | -0.618631 | -3.136631 | -0.237687 |
| C | 2.791945 | -1.557625 | -0.237687 |
| C | 0.618631 | -3.136631 | -0.237687 |
| C | -1.343182 | 2.901210 | -0.237687 |
| C | -2.344148 | 2.173965 | -0.237687 |

$C_{20}$ Cage $C_{2h}$

| | | | |
|---|---|---|---|
| C | 0.374588 | 2.045994 | 0.000000 |
| C | -0.374588 | -2.045994 | 0.000000 |
| C | 1.579782 | 1.352337 | 0.000000 |
| C | 0.380275 | -1.569714 | 1.173775 |
| C | -0.380275 | 1.569714 | 1.173775 |
| C | -1.579782 | -1.352337 | 0.000000 |
| C | -0.380275 | 1.569714 | -1.173775 |
| C | 0.380275 | -1.569714 | -1.173775 |
| C | -1.563187 | 0.899197 | -0.716790 |
| C | -0.380275 | -0.661143 | -1.942085 |
| C | 1.548134 | 0.460514 | -1.173924 |
| C | 1.563187 | -0.899197 | 0.716790 |
| C | 0.380275 | 0.661143 | 1.942085 |
| C | -1.548134 | -0.460514 | 1.173924 |
| C | 1.563187 | -0.899197 | -0.716790 |
| C | 0.380275 | 0.661143 | -1.942085 |
| C | -1.548134 | -0.460514 | -1.173924 |
| C | -1.563187 | 0.899197 | 0.716790 |
| C | -0.380275 | -0.661143 | 1.942085 |
| C | 1.548134 | 0.460514 | 1.173924 |

$C_{20}$ Cage $C_i$

| | | | |
|---|---|---|---|
| C | 1.776873 | 0.729819 | 0.180200 |

| | | | |
|---|---|---|---|
| C | -1.776873 | -0.729819 | -0.180200 |
| C | 1.322564 | 0.207697 | 1.435613 |
| C | -1.322564 | -0.207697 | -1.435613 |
| C | 0.139768 | 0.919285 | 1.836484 |
| C | -0.139768 | -0.919285 | -1.836484 |
| C | -0.156206 | 1.920266 | 0.752637 |
| C | 0.156206 | -1.920266 | -0.752637 |
| C | -0.863929 | -1.747844 | 0.249924 |
| C | 0.863929 | 1.747844 | -0.249924 |
| C | -1.770257 | 0.329781 | 0.785663 |
| C | 1.770257 | -0.329781 | -0.785663 |
| C | 1.061954 | -1.200457 | 1.289537 |
| C | -1.061954 | 1.200457 | -1.289537 |
| C | -0.888633 | -0.024590 | 1.862756 |
| C | 0.888633 | 0.024590 | -1.862756 |
| C | -1.354407 | 1.550381 | 0.141662 |
| C | 1.354407 | -1.550381 | -0.141662 |
| C | -0.303948 | -1.371092 | 1.519586 |
| C | 0.303948 | 1.371092 | -1.519586 |

$C_{20}$ Cage $D_{2h}$

| | | | |
|---|---|---|---|
| C | -1.959980 | 0.000000 | 0.695496 |
| C | 1.959980 | 0.000000 | -0.695496 |
| C | -1.959980 | 0.000000 | -0.695496 |
| C | 1.170893 | 1.173662 | -1.112266 |
| C | -1.170893 | 1.173662 | 1.112266 |
| C | 1.959980 | 0.000000 | 0.695496 |
| C | -1.170893 | -1.173662 | 1.112266 |
| C | 1.170893 | -1.173662 | -1.112266 |
| C | 0.000000 | -0.716938 | 1.803688 |
| C | 0.762971 | -1.942394 | 0.000000 |
| C | -1.170893 | -1.173662 | -1.112266 |
| C | 0.000000 | 0.716938 | -1.803688 |
| C | -0.762971 | 1.942394 | 0.000000 |
| C | 1.170893 | 1.173662 | 1.112266 |
| C | 0.000000 | -0.716938 | -1.803688 |
| C | -0.762971 | -1.942394 | 0.000000 |
| C | 1.170893 | -1.173662 | 1.112266 |
| C | 0.000000 | 0.716938 | 1.803688 |
| C | 0.762971 | 1.942394 | 0.000000 |
| C | -1.170893 | 1.173662 | -1.112266 |

$C_{20}$ Cage $D_{3h}$

| | | | |
|---|---|---|---|
| C | 0.000000 | 0.000000 | 1.928162 |
| C | 0.000000 | 0.000000 | -1.928162 |
| C | -1.164573 | 0.672366 | 1.431482 |
| C | 1.164573 | -0.672366 | -1.431482 |
| C | -0.752755 | 1.808353 | 0.650390 |
| C | 0.752755 | -1.808353 | -0.650390 |
| C | 0.752755 | 1.808353 | 0.650390 |

| | | | |
|---|---|---|---|
| C | -0.752755 | -1.808353 | -0.650390 |
| C | -1.164573 | -0.672366 | -1.431482 |
| C | 1.164573 | 0.672366 | 1.431482 |
| C | 0.000000 | 1.344733 | -1.431482 |
| C | 0.000000 | -1.344733 | 1.431482 |
| C | -1.942457 | -0.252272 | 0.650390 |
| C | 1.942457 | 0.252272 | -0.650390 |
| C | -1.189702 | 1.556081 | -0.650390 |
| C | 1.189702 | -1.556081 | 0.650390 |
| C | 1.189702 | 1.556081 | -0.650390 |
| C | -1.189702 | -1.556081 | 0.650390 |
| C | -1.942457 | 0.252272 | -0.650390 |
| C | 1.942457 | -0.252272 | 0.650390 |

$C_{20}$ Ring $C_{10h}$

| | | | |
|---|---|---|---|
| C | 1.211232 | 3.918783 | 0.000000 |
| C | 0.000000 | 4.101480 | 0.000000 |
| C | -1.323496 | 3.882306 | 0.000000 |
| C | -2.410789 | 3.318167 | 0.000000 |
| C | -3.352693 | 2.362921 | 0.000000 |
| C | -3.900739 | 1.267427 | 0.000000 |
| C | -4.101275 | -0.059020 | 0.000000 |
| C | -3.900739 | -1.267427 | 0.000000 |
| C | -3.283310 | -2.458418 | 0.000000 |
| C | -2.410789 | -3.318167 | 0.000000 |
| C | -1.211232 | -3.918783 | 0.000000 |
| C | 0.000000 | -4.101480 | 0.000000 |
| C | 1.323496 | -3.882306 | 0.000000 |
| C | 2.410789 | -3.318167 | 0.000000 |
| C | 3.352693 | -2.362921 | 0.000000 |
| C | 3.900739 | -1.267427 | 0.000000 |
| C | 4.101275 | 0.059020 | 0.000000 |
| C | 3.900739 | 1.267427 | 0.000000 |
| C | 3.283310 | 2.458418 | 0.000000 |
| C | 2.410789 | 3.318167 | 0.000000 |

$C_{24}$ Cage $O_h$

| | | | |
|---|---|---|---|
| C | 0.000000 | 1.048369 | 2.014322 |
| C | 0.000000 | -1.048369 | 2.014322 |
| C | 1.048369 | 0.000000 | 2.014322 |
| C | -1.048369 | 0.000000 | 2.014322 |
| C | 0.000000 | 2.014322 | 1.048369 |
| C | 0.000000 | 2.014322 | -1.048369 |
| C | 1.048369 | 2.014322 | 0.000000 |
| C | -1.048369 | 2.014322 | 0.000000 |
| C | 0.000000 | 1.048369 | -2.014322 |
| C | 0.000000 | -1.048369 | -2.014322 |
| C | 1.048369 | 0.000000 | -2.014322 |
| C | -1.048369 | 0.000000 | -2.014322 |
| C | 0.000000 | -2.014322 | 1.048369 |

| | | | |
|---|---|---|---|
| C | 0.000000 | -2.014322 | -1.048369 |
| C | 1.048369 | -2.014322 | 0.000000 |
| C | -1.048369 | -2.014322 | 0.000000 |
| C | 2.014322 | 0.000000 | 1.048369 |
| C | 2.014322 | 1.048369 | 0.000000 |
| C | 2.014322 | 0.000000 | -1.048369 |
| C | 2.014322 | -1.048369 | 0.000000 |
| C | -2.014322 | 0.000000 | 1.048369 |
| C | -2.014322 | 1.048369 | 0.000000 |
| C | -2.014322 | 0.000000 | -1.048369 |
| C | -2.014322 | -1.048369 | 0.000000 |

$C_{24}$ Cage $D_{3d}$

| | | | |
|---|---|---|---|
| C | -0.563041 | 2.215237 | 0.378349 |
| C | -2.199972 | 0.620011 | 0.378349 |
| C | -1.636931 | -1.595226 | 0.378349 |
| C | 0.563041 | -2.215237 | 0.378349 |
| C | 2.199972 | -0.620011 | 0.378349 |
| C | 1.636931 | 1.595226 | 0.378349 |
| C | 2.199972 | 0.620011 | -0.378349 |
| C | 0.563041 | 2.215237 | -0.378349 |
| C | -1.636931 | 1.595226 | -0.378349 |
| C | -2.199972 | -0.620011 | -0.378349 |
| C | -0.563041 | -2.215237 | -0.378349 |
| C | 1.636931 | -1.595226 | -0.378349 |
| C | -0.338218 | 1.373041 | 1.624431 |
| C | -1.358197 | 0.393615 | 1.624431 |
| C | -1.019979 | -0.979426 | 1.624431 |
| C | 0.338218 | -1.373041 | 1.624431 |
| C | 1.358197 | -0.393615 | 1.624431 |
| C | 1.019979 | 0.979426 | 1.624431 |
| C | 1.358197 | 0.393615 | -1.624431 |
| C | 0.338218 | 1.373041 | -1.624431 |
| C | -1.019979 | 0.979426 | -1.624431 |
| C | -1.358197 | -0.393615 | -1.624431 |
| C | -0.338218 | -1.373041 | -1.624431 |
| C | 1.019979 | -0.979426 | -1.624431 |

$C_{24}$ Corona $D_{6h}$

| | | | |
|---|---|---|---|
| C | 0.000000 | 0.000000 | 1.440593 |
| C | 0.000000 | 1.247598 | 0.720333 |
| C | 0.000000 | 1.247598 | -0.720333 |
| C | 0.000000 | 0.000000 | -1.440593 |
| C | 0.000000 | -1.247598 | -0.720333 |
| C | 0.000000 | -1.247598 | 0.720333 |
| C | 0.000000 | 0.000000 | 2.917240 |
| C | 0.000000 | 2.526509 | 1.458723 |
| C | 0.000000 | 2.526509 | -1.458723 |
| C | 0.000000 | 0.000000 | -2.917240 |
| C | 0.000000 | -2.526509 | -1.458723 |

| | | | |
|---|---|---|---|
| C | 0.000000 | -2.526509 | 1.458723 |
| C | 0.000000 | 1.277541 | 3.440833 |
| C | 0.000000 | 3.618623 | 0.614014 |
| C | 0.000000 | 2.341063 | -2.826850 |
| C | 0.000000 | -1.277541 | -3.440833 |
| C | 0.000000 | -3.618623 | -0.614014 |
| C | 0.000000 | -2.341063 | 2.826850 |
| C | 0.000000 | -1.277541 | 3.440833 |
| C | 0.000000 | 2.341063 | 2.826850 |
| C | 0.000000 | 3.618623 | -0.614014 |
| C | 0.000000 | 1.277541 | -3.440833 |
| C | 0.000000 | -2.341063 | -2.826850 |
| C | 0.000000 | -3.618623 | 0.614014 |

$C_{24}$ Ring $C_{12h}$

| | | | |
|---|---|---|---|
| C | 0.613780 | 4.871844 | 0.000000 |
| C | 2.967471 | 3.912251 | 0.000000 |
| C | 4.526031 | 1.904373 | 0.000000 |
| C | 4.871844 | -0.613780 | 0.000000 |
| C | 3.912251 | -2.967471 | 0.000000 |
| C | 1.904373 | -4.526031 | 0.000000 |
| C | -0.613780 | -4.871844 | 0.000000 |
| C | -2.967471 | -3.912251 | 0.000000 |
| C | -4.526031 | -1.904373 | 0.000000 |
| C | -4.871844 | 0.613780 | 0.000000 |
| C | -3.912251 | 2.967471 | 0.000000 |
| C | -1.904373 | 4.526031 | 0.000000 |
| C | 1.904373 | 4.526031 | 0.000000 |
| C | 3.912251 | 2.967471 | 0.000000 |
| C | 4.871844 | 0.613780 | 0.000000 |
| C | 4.526031 | -1.904373 | 0.000000 |
| C | 2.967471 | -3.912251 | 0.000000 |
| C | 0.613780 | -4.871844 | 0.000000 |
| C | -1.904373 | -4.526031 | 0.000000 |
| C | -3.912251 | -2.967471 | 0.000000 |
| C | -4.871844 | -0.613780 | 0.000000 |
| C | -4.526031 | 1.904373 | 0.000000 |
| C | -2.967471 | 3.912251 | 0.000000 |
| C | -0.613780 | 4.871844 | 0.000000 |
